# Supplementary material for: Semantically Distributed Robust Optimization for Vision-and-Language Inference
Source: arXiv:2110.07165 source file (2022-03-14)
Supplement: Supplementary file 1 [file violin_text_attack.tex]

\begin{table}[t]
    \centering
    \small 
    {\resizebox{\linewidth}{!}{
    \begin{tabular}{@{}p{15mm} ccccccc@{}}
        \toprule
        % \multirow{2}{*}{\textbf{Model}} & \multicolumn{7}{c}{\textbf{Text Attack Categories}} \\
        \textbf{Model} & \textbf{CLARE} & \textbf{CharSwap} & \textbf{CheckList} & \textbf{EDA} & \textbf{Emb} & \textbf{WordNet} & \textbf{Avg.}\\
        \midrule
        HERO          & 66.08  & 63.00 & 68.58 & 60.89 & 63.81 & 63.38 & 64.29 \\
        HERO{+}SDRO   & 68.70 & 64.95 & 68.96 & 61.32 & 65.54 & 64.61 & 65.68 \\
        \bottomrule 
    \end{tabular}
    }
    }
    \caption{Performance on VIOLIN ``text-attack'' set created using augmentation techniques from Text-Attack.}
    \label{tab:violin_text_attack}
\end{table}
