# Supplementary material for: Semantically Distributed Robust Optimization for Vision-and-Language Inference
Source: arXiv:2110.07165 source file (2022-03-14)
Supplement: Supplementary file 2 [file vqa_textattack.tex]

\begin{table}[ht]
    \centering
    \small 
    {\resizebox{\linewidth}{!}{
    \begin{tabular}{@{}p{15mm} ccccccc@{}}
        \toprule
        % \multirow{2}{*}{\textbf{Model}} & \multicolumn{7}{c}{\textbf{Text Attack Categories}} \\
        \textbf{Model} & \textbf{CLARE} & \textbf{CharSwap} & \textbf{CheckList} & \textbf{EDA} & \textbf{Emb} & \textbf{WordNet} & \textbf{Avg.}\\
        \midrule 
        UN          & 80.82 & 75.74 & 82.46 & 72.74 & 76.94 & 76.85 & 77.59 \\
        UN + SDRO   & 83.57 & 77.72 & 84.43 & 74.05 & 80.31 & 73.38 & 78.91 \\
        \midrule 
        VI          & 80.49 & 75.74 & 84.87 & 74.64 & 78.63 & 76.39 & 78.45 \\
        VI + SDRO   & 85.99 & 84.52 & 84.10 & 87.02 & 84.25 & 84.03 & 84.99 \\
        \bottomrule
    \end{tabular}
    }
    }
    \caption{Performance on VQA-Yes/No ``text-attack'' set created using augmentation techniques from Text-Attack.}
    \label{tab:vqa_text_attack}
\end{table}
